# Supplementary material for: Life and Death of a Thin Liquid Film
Source: arXiv:2311.00419 source file (2023-11-01)
Supplement: Supplementary file 1 [file SI.pdf]

# Supplementary Information: Life and Death of a Thin Liquid Film

Muhammad Rizwanur Rahman[1], Li Shen[1], James P. Ewen [1], D. M. Heyes[1], Daniele Dini[1], and E. R. Smith[2]

[1]Department of Mechanical Engineering, Imperial College London, South Kensington Campus, London SW7 2AZ, United Kingdom
[2]Department of Mechanical and Aerospace Engineering, Brunel University London, Uxbridge UB8 3PH, United Kingdom

November 1, 2023

## Contents

**1 Self-similar growth** **2**

**2 Rupture Memory** **4**

**3 Formation of a nucleus** **5**

**4 Neighbor effect on the propagation of rupture** **6**

**5 Cahn-Hilliard Theory** **9**

# 1 Self-similar growth

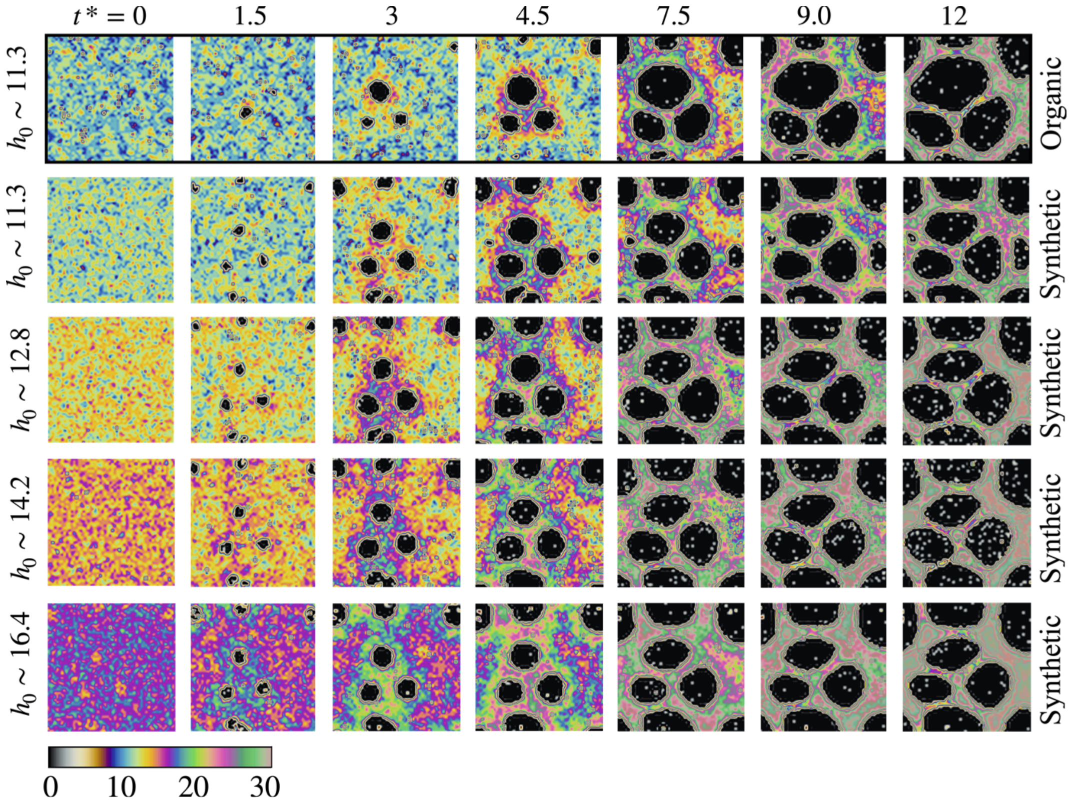


**Supplementary Figure 1**: Spontaneously formed (top row) and synthetically generated (other rows) nuclei on films of various thicknesses show similar evolution pattern over non-dimensional time, $t^* = (t - t_n)/\tau_i$; $\tau_i$ is the inertial time scale. The synthetic nuclei were generated in a controlled way to maintain $R_0/h_0 \sim 0.8$.

The locations of the center of the spontaneously formed nuclei of 1st row in Supplementary Fig. 1 on a film of thickness, $h_0 \sim 11.3$ were identified and, were later used to generate synthetic nuclei at the same locations on thicker films. The time-sequence of spontaneous nucleus formation was removed by nucleating the holes at the same time. While generating the synthetic nuclei, the initial radii were chosen such that $R_0/h_0 \sim 0.85$. Once formed, the nuclei grow at the so-called Taylor-Culick speed which depends on the film thickness, until the neighboring nuclei are grown enough to start interacting with each other, when the growth slows down and deflect from the linear Taylor-Culick speed. The thickness dependence of the growth dynamics is removed by normalizing the time by the inertial time scale, $\tau_i = \sqrt{\rho h_0^3/2\gamma}$. Irrespective of the initial thickness, $h_0$, the nuclei in each of the films grow in the exact same fashion, except for $h_0 \sim 11.3$ where a new nucleus emerges spontaneously within the simulated time-window. Supplementary Figure 2 shows later stages of growth where nuclei coalesce leading to fragmentation of teh film into droplets.

Apparent from these results, if the nucleation time and the location of nucleation were same, the evolution of the films of varied $h_0$ would be identical. Only the spatio-temporal distribution of the of nucleation can cause any different pattern.

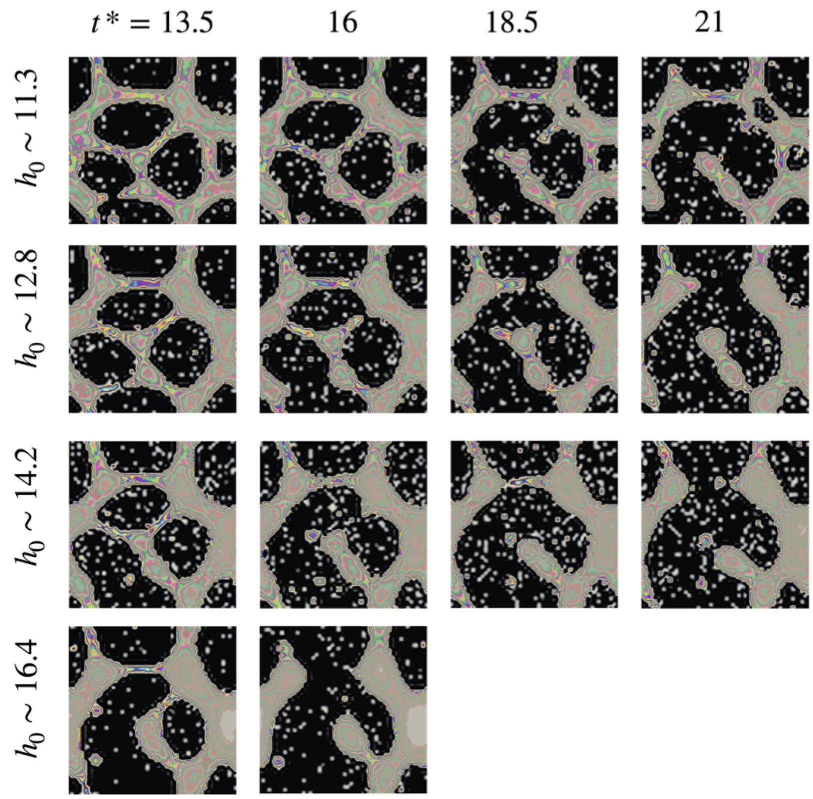


**Supplementary Figure 2**: Transition to coalescence regime: nuclei in a relatively thicker film coalesce earlier than those in a thinner film.

The 'undisturbed' growth of a nucleus is highly effected once it come to close proximity of surrounding nuclei. The scarceness of space to grow, and the increasing thickness of the surrounding liquid between the neighbors frustrates the growth and the nucleus is squeezed - indicated by the deviation of the circularity of its shape. When two neighboring nuclei come in close contact to each other, the likelihood of coalescence increases with their sizes as two larger nuclei will share larger contact area in the direction normal to the film-surface. The liquid trapped within the two nuclei can then be thought of another freely suspended film but spans across the direction along the thickness of the parent film. As the lateral dimension of this 'trapped' film increases both with the film thickness and the size of the nuclei, larger nuclei and in thicker films, are more prone to rupture as compared to smaller nuclei and thinner films. Indeed, these trapped films are essentially a fractal version of the parent film, so one can expect similar behavior, but in a smaller length and time scale. As seen from the top row of Supplementary Fig. 2, the growth of the nuclei, their coalescence and subsequent growth results in long liquid threads[1], which can be

considered as films along the normal direction, these soon break due to the Rayleigh instability.

## 2 Rupture Memory

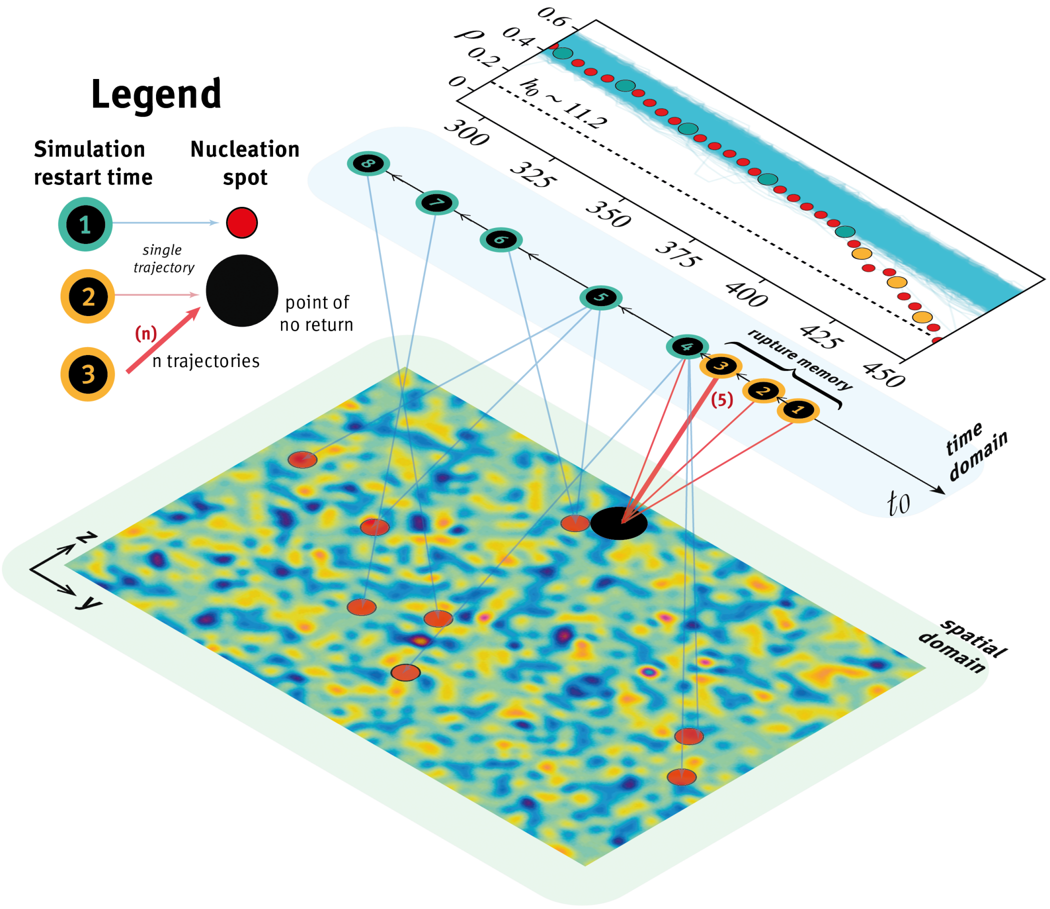


**Supplementary Figure 3**: In addition to the film detailed in the manuscript Figure 3, a repeat examination of an independent simulations (which originally nucleates at $t \sim 450$) is carried out (bottom density plot and the related connection lines). Similar to what is described in the MS, connection lines to the nuclei are red when a restarted case nucleates at the same location as of the original film (white circle on the film), and blue otherwise.

Supplementary Figure 3 shows the memory-effect of film rupture. Multiple independent simulations nucleate at the identical spot until approximately $t_n \sim 401$. However, delving further back in time (i.e., $t < 401$), discrepancies arise both in spatial distribution and nucleation timing. One might speculate whether this discrepancy is solely attributed to a local density threshold. It is important to note that the memory window differs between the two investigated cases, but in both

cases, the span of the memory window exceeds the numerical correlation time of the molecular simulation.

# 3 Formation of a nucleus

Supplementary Fig. 4 (a), shows the temporal evolution of the local thickness at the center of a rupture site over non-dimensional time, $\tilde{t} = (t - t_n)/\tau_i$, where $t_n$ is the time of nucleation, $\tau_i$ is the inertial time scale, and defined as $\tau_i = \rho h_0^3/2\gamma$. The film gradually thins over time, and once its thickness reaches $\sim 10$, the rate of thinning is accelerated leading to the formation of a nucleus - as seen in the shaded region of the figure. Supplementary Figure 4 (b) presents the radial and thickness-averaged local density profile of a site nucleating at time $t_n$, situated at $r = 0$. Notably, the initiation of local thinning (or dimple formation) is evident from the plot. Panel (c), which is presented in the main text as well, offers a reconstruction of the nucleus-proximal region through rotation of the density profile presented in panel (c), see Supplementary Fig. 5 for more instances.

The time of the first nucleation event, denoted as $t_n$, exhibits pronounced sensitivity to the film thickness, $h_0$. This relationship is seen in Fig. 4 (d), which clearly illustrates that $t_n$ increases approximately with the third power of $h_0$, within the simulation statistics. Ruckenstein and Jain [2] studied the rupture of the pure thin film free from surface active agents, and argued that the out-of-phase fluctuations at the upper and lower surfaces lead to the most rapid rupture. Considering the out-of-phase perturbations, the rupture time, $\tau$ can be related to the initial film thickness as[2]: $\tau \approx \frac{6\pi\mu\bar{h}^3}{\mathcal{H}}$, here, $\mathcal{H}$ is the Hamaker constant, and $\bar{h}$ is the average film thickness. It is problematic to measure an accurate Hamaker constant for thin films, and the possible dependence of this constant on the film thickness cannot be ruled out, which leads to uncertainties in the prediction of the rupture time, as does the approximation of uniform film thickness.

The literature establishes that the presence of impurities or surfactants contribute to heightened film elasticity, imparting significant stabilization. Under such conditions, the assumption of a substantial $\Gamma d\gamma/d\Gamma$ (where $\Gamma$ is the surfactant concentration at the surface) leads to a more conservative assessment of the rupture time. This notion aligns with the formulation proposed by Vrij and Overbeek [3], which estimates $\tau \approx h_0^5$.

Supplementary Figure 4 (e) shows the temporal evolution of the number of nuclei across a film of thickness, $h_0 \sim 10$ for three independent simulations. It is evident that for thinner films, nucleation occurs at multiple sites within a relatively short time period, and the film quickly enters the coalescence regime, and the nuclei start to merge into bigger nuclei. Supplementary Figure 4 (f) shows how the areal density (the ratio of the maximum number of nuclei to the lateral area of the film) of the nuclei decreases with increasing film thickness, just as was carried out in a study of liquid crystal films[4]. The solid line denotes a fit to the data according to the scaling law, i.e., $\rho_N \sim h_0^{-4}$, proposed in earlier theoretical and experimental studies[5,6].

Note here, these spontaneous rupture sites (and the thinnest parts in the film) emerged at varied locations across the film, and did not cluster only around the film edge as reported in a recent experimental study on colloidal films[7].

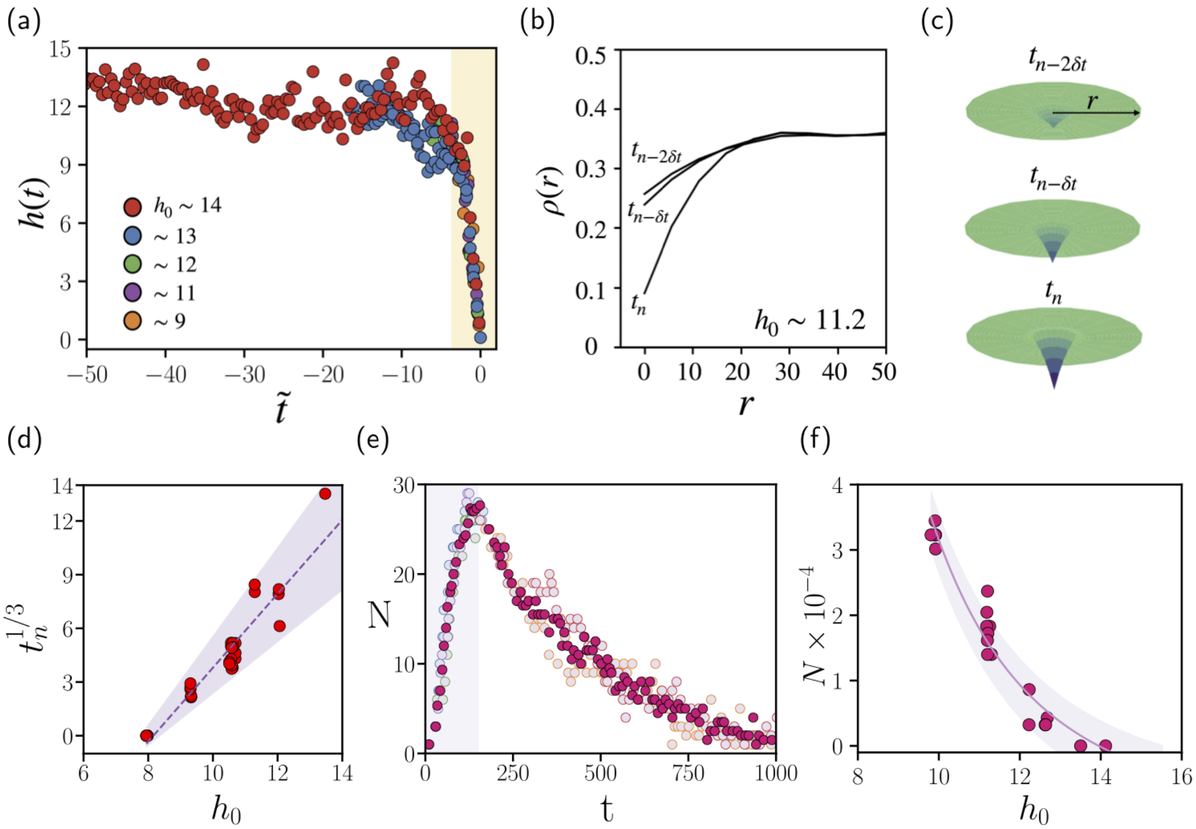


**Supplementary Figure 4**: Temporal variation of the thickness of the center of a nucleus that forms at time, $\tilde{t} = 0$, where, $\tilde{t} = (t - t_n)/\tau_i$ with $t_n$ the time of nucleation, and $\tau_i$ the inertial time scale. (b) radial (and thickness) averaged density profile around a nucleus at times closer to its nucleation for a film with $h_0 \sim 11.2$, $r = 0$ is the center of the nucleus, and $\delta t = 25$ units of MD time. (c) A full revolution of the density profiles around the axis through the nucleus-center at t $=$ $t_{n-2\delta}$, $t_{n-\delta}$ and $t_n$. (d) $t_n$ varies with the third power of the film thickness, $h_0$. Multiple independent simulations were carried out for each thickness. Symbols denote individual simulations, and the dashed line shows fitting to the data according to $t_n \propto h_0^3$. (e) Number of nuclei, $N$ formed on a film of thickness, $h_0 \sim 10$ over time. Beyond the shaded region, coalescence starts (shaded region) and $N$ starts decreasing. Faint circles show data of individual simulations, filled solid circles denote averaged data. (f) Areal density of nuclei (per MD unit area) as a function of $h_0$. Multiple independent simulations were conducted for each thickness. The line shows a $N \propto h_0^{-4}$ fit to the data.

# 4 Neighbor effect on the propagation of rupture

It is rare, if not impossible, to find a film where the rupture sites are isolated. Indeed, and as can be seen in the films presented in the figures of the manuscript, multiple sites on the film rupture

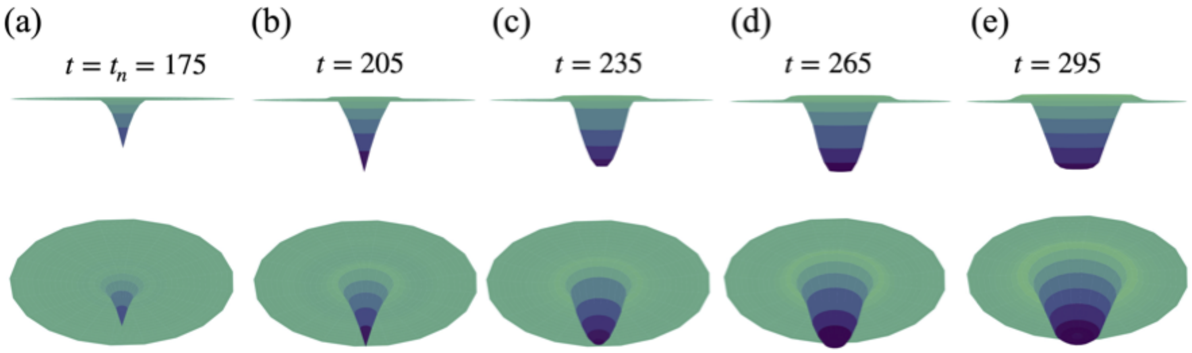


**Supplementary Figure 5**: The evolution of the density profile as a nucleus grows. Top panel shows side view of the revolved profile which evidences the accumulation of liquid around the nucleus forming a rim. The bottom panel shows same profile from a different elevation angle.

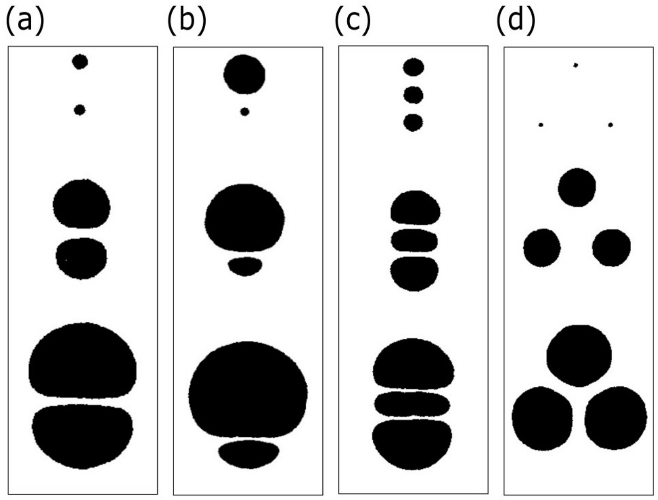


**Supplementary Figure 6**: Effect of neighbors on the shape and size of a nucleus: two nuclei where one nucleates (a) slightly earlier than the other, (b) substantially earlier than the other. Three nuclei that nucleate at the same time located (c) on the same axis, (d) on the vertices of an equilateral triangle.

almost simultaneously. For relatively thicker films, the rupture sites are more sparsely distributed than for thinner films, but upon expansion, the rim of these distant nuclei come close to each other effecting the growth of other nuclei. As can be seen from Supplementary Fig. 6 (a-d), the growth of each of the nuclei is effected due to the presence of the neighbors. And, such effect is seen to be a function of the relative size, location and the number of neighbors. In panel (a), the two nucleus share nearly equal effect from each other, but in panel (b), where one nucleus is significantly aged (hence, larger) than the other, the larger nucleus is seen to push the smaller one (can be realized

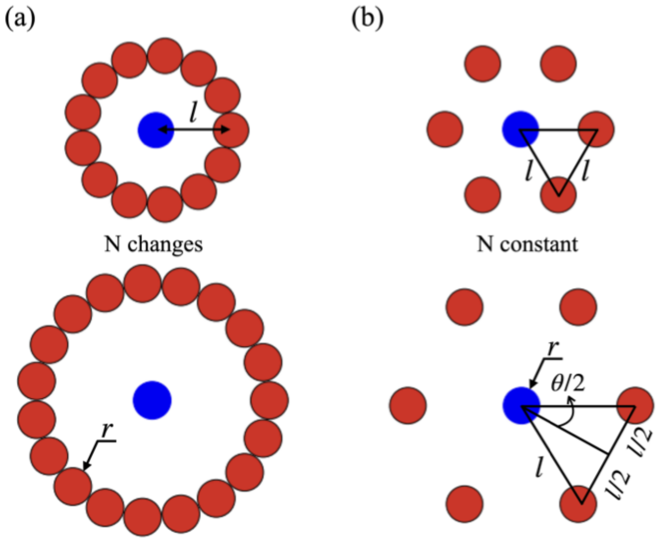


**Supplementary Figure 7**: Schematic of a central nucleus surrounded by neighbor nuclei. (a) densely packed case where neighbors touch but do not overlap onto each other, (b) center-to-center distance between two neighbors equals the center-to-center distance between the central nucleus and the neighbor nucleus. For both panels, the distance between the central and the neighbor nuclei is increased by nearly 50%. For (a) $N = 6$ only when $l = 2r$, whereas, for (b) irrespective of the magnitude of $l$, $N = 6$.

from an increase of their center-to-center distance). In panel (c), the greatest impact is on the central nucleus which is squeezed by the two side-nuclei. In contrast, in panel (d) each of the three nuclei effect each-other equally.

It can be realized that depending on the time and location of nucleation, an infinite set of possibilities may occur. In this study, we systematically examine few simplified but representative cases that presents an understanding of the over-all neighbor effects.

## Maximum number of neighbors

For simplicity, we assume $N$ nearest-neighbors nuclei each of radius, $r$ surround a central nucleus, $C_c$ of radius $R$, and $R(t_0) = r(t_0)$. If the $nn$ nuclei are uniformly located at a distance $l$ from the center of $C_c$, the maximum possible number of neighbors of radius, $r$ can be obtained as:

$$N_{\max} = \frac{\pi}{\sin^{-1}(r/l)} - 1 \tag{1}$$

This, however, refers to a situation where the neighbors are densely packed, i.e., they touches their side nuclei without overlapping, see Supplementary Fig.7 (a). Note, in situation like this, $N_{\max}$ varies with the center-to-center distance, $l$, i.e., $N_{\max} = N(l)$. Further, since the neighbors

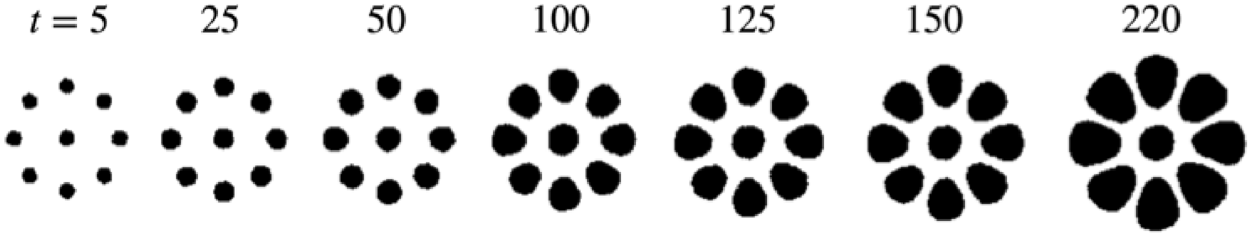


**Supplementary Figure 8**: Evolution of a central nucleus surrounded by 8 neighbor nuclei initially located at equal distance from the central nucleus. After initial growth, the central nucleus is seen to suffocate to grow and eventually reaches a stagnant shape. Time is in MD units.

themselves would grow over time, if such a situation arises, they will rather coalesce with each other before the central nucleus is effected.

A different arrangement is shown in the top and bottom rows of panel (b), where the distance between the central and any of the neighbor nuclei is equal to the distance of any two neighbor nuclei. If such a condition is imposed, (i) the neighbor nuclei would affect each-other only when they also start affecting the central nucleus, and (ii) any pre-mature coalescence can be avoided. With such an arrangement, the maximum number of neighbor nuclei can be obtained from the geometry as shown in Fig.7 (b):

$$N_{\max} = \frac{\pi}{\sin^{-1}\left(\frac{l/2}{l}\right)} \tag{2}$$

As evident from Eq. 2, $N_{\max}$ is independent of $l$ and assumes a value of 6.

This is portrayed in Supplementary Fig. 8 where 8 neighbor nuclei surrounds a central nucleus. Initially, all the nuclei are seen to grow in similar fashion. However, one can notice that after $t \geq 100$, the growth of the central nucleus is slowed and later almost stopped, while the neighbour nuclei keep growing and effecting each other.

# 5 Cahn-Hilliard Theory

The free energy associated film rupture can be conveniently dissected into two fundamental components: the energy attributed to the interface and the energy barrier. This can be captured effectively using the Cahn-Hilliard (C-H) system which provides a phenomenological framework that characterizes the dynamics of thin films as the gradient flow of an energy function expressed as $J[u] = \int \left(\frac{1}{2}\sigma \left|\nabla u\right|^2 + F'(u)\right) du$, where $F'(u)$ is the bulk free energy (energy barrier), the gradient term represents the energy of the interface which separates the phases and $\sigma$ denotes the relative importance of the bulk and interfacial energies. Although commonly referred to as a 'phenomenological theory', the Cahn-Hilliard (C-H) framework can, in fact, be derived from the Navier-Stokes equations through a long-wave asymptotic expansion[8,9].

Given the established relationship between the Navier-Stokes equations and the Boltzmann

kinetic theory[10], it logically extends to derive the Cahn-Hilliard (C-H) framework from kinetic theory[11]. Therefore, we no longer view C-H as a phenomenological surrogate for the spinodal rupture process but a first order equivalent formulation in line with the Chapman-Enskog expansion[10] of the generalised Boltzmann equation at the Navier-Stokes order. In this sense, spinodal dewetting, homogeneous and heterogeneous nucleation are all manifestations of the C-H system with varying $\sigma$ and $F$, or due to the differences in initial conditions. In other words, they represent different modes of the same equation, showcasing how localized changes in free energy, either in space or in time, as well as the relative significance of interfacial and bulk energy, lead to these diverse phenomena.

# References


[1] Ruhi Verma and Ashutosh Sharma. Defect sensitivity in instability and dewetting of thin liquid films: Two regimes of spinodal dewetting. *Industrial & Engineering Chemistry Research*, 46(10):3108–3118, 2007.

[2] Eli Ruckenstein and Rakesh K Jain. Spontaneous rupture of thin liquid films. *Journal of the Chemical Society, Faraday Transactions 2: Molecular and Chemical Physics*, 70:132–147, 1974.

[3] A Vrij and J Th G Overbeek. Rupture of thin liquid films due to spontaneous fluctuations in thickness. *Journal of the American Chemical Society*, 90(12):3074–3078, 1968.

[4] Trung Dac Nguyen, Jan-Michael Y Carrillo, Michael A Matheson, and W Michael Brown. Rupture mechanism of liquid crystal thin films realized by large-scale molecular simulations. *Nanoscale*, 6(6):3083–3096, 2014.

[5] Günter Reiter. Dewetting of thin polymer films. *Physical Review Letters*, 68(1):75, 1992.

[6] Ashutosh Sharma and Günter Reiter. Instability of thin polymer films on coated substrates: rupture, dewetting, and drop formation. *Journal of Colloid and Interface Science*, 178(2): 383–399, 1996.

[7] Phalguni Shah, Eleanor Ward, Srishti Arora, and Michelle M Driscoll. Rupture dynamics of flat colloidal films. *Physical Review Fluids*, 8(2):024002, 2023.

[8] Alexander Oron, Stephen H Davis, and S George Bankoff. Long-scale evolution of thin liquid films. *Reviews of modern physics*, 69(3):931, 1997.

[9] Li Shen, Fabian Denner, Neal Morgan, Berend van Wachem, and Daniele Dini. Transient structures in rupturing thin films: Marangoni-induced symmetry-breaking pattern formation in viscous fluids. *Science Advances*, 6(28):eabb0597, 2020.

[10] Sydney Chapman and TG Cowling. *The Mathematical Theory of Non-Uniform Gases*. Cambridge Mathematical Library. Cambridge University Press, third edition, 1970.

[11] Vincent Giovangigli. Kinetic derivation of cahn-hilliard fluid models. *Physical Review E*, 104 (5):054109, 2021.
